# Supplementary material for: A Multimodal Target-Source Classifier with Attention Branches to Understand Ambiguous Instructions for Fetching Daily Objects
Source: arXiv:1912.10675 source file (2019-12-25)
Supplement: Supplementary file 1 [file appendix.tex]

%\begin{appendices}


%\end{appendices}
